# Supplementary material for: Spin interactions and magnetic order in the iron oxychalcogenides BaFe2Q2O
Source: arXiv:1902.09035 source file (2019-05-29)
Supplement: Supplementary file 1 [file 180219b_BaFe2Q2O_supplementary_material.pdf]

**$BaFe_2Q_2O$ *Q* = S, Se Supplementary materials:**

**SM1 Magnetic measurements:**

SM1.1 Field-sweep data for $BaFe_2S_2O$ at 10 K

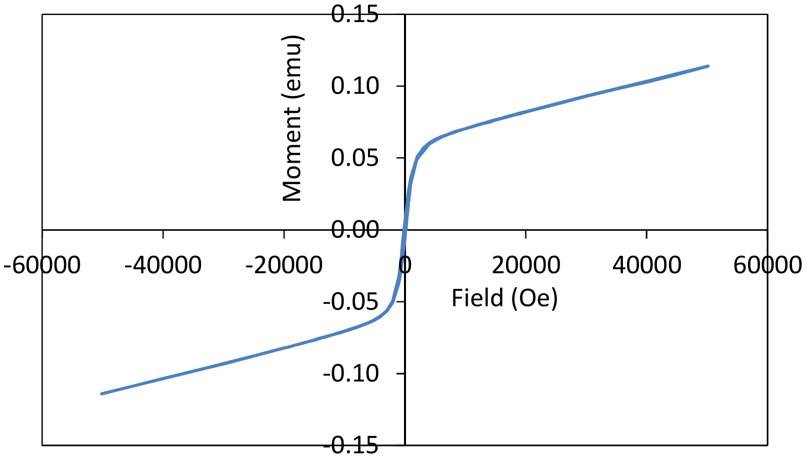


Figure SM1.1 Field-sweep data for $BaFe_2S_2O$ at 10 K

SM1.2 FC and ZFC data for $BaFe_2S_2O$ in 55000 Oe applied field

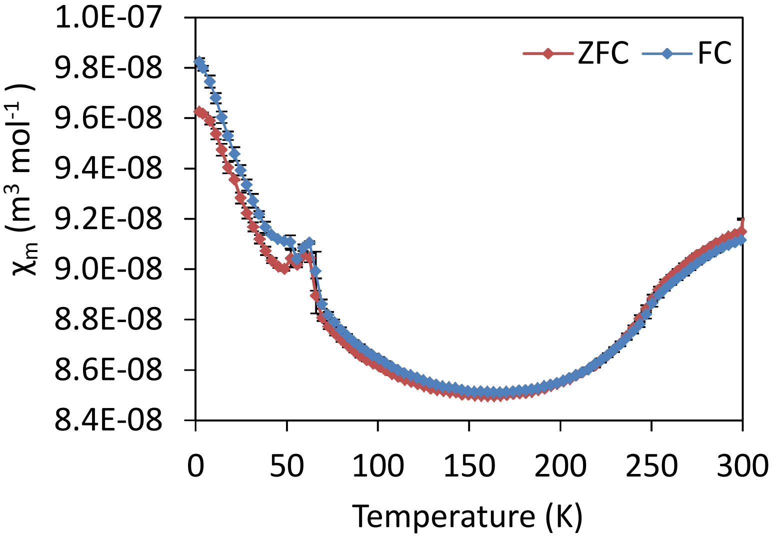


Figure SM1.2 Field-cooled and zero-field-cooled magnetisation data for collected for $BaFe_2S_2O$ in 55000 Oe applied field.

SM1.3 FC and ZFC data for $BaFe_2S_2O$ in 45000 Oe applied field

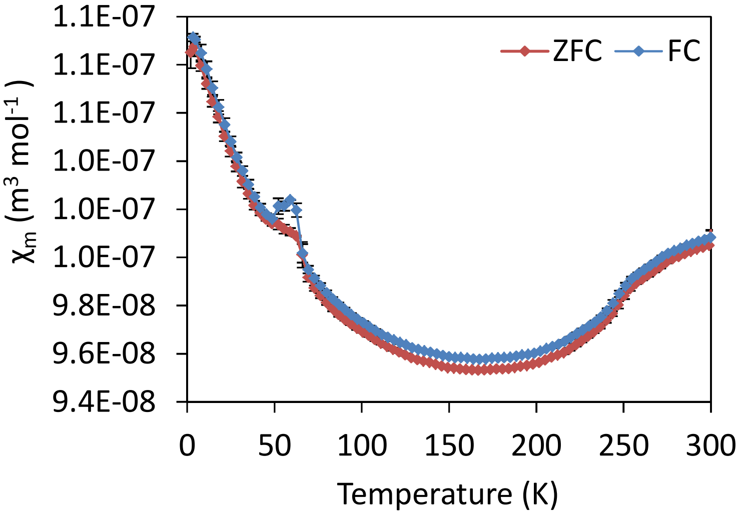


Figure SM1.3 Field-cooled and zero-field-cooled magnetisation data for collected for $BaFe_2S_2O$ in 45000 Oe applied field.

SM1.4 FC and ZFC data for $BaFe_2Se_2O$ in 1000 Oe field, showing comparable magnetic susceptibility to that reported by Lei et al.[1]

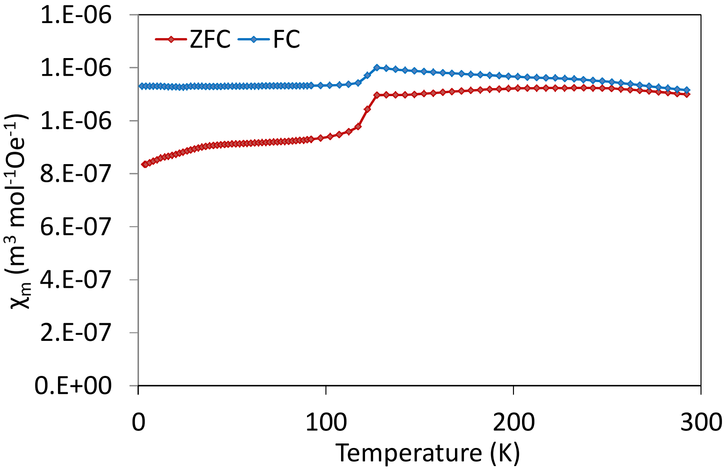


Figure SM1.4 Field-cooled and zero-field-cooled magnetisation data for collected for $BaFe_2Se_2O$ in 1000 Oe applied field.

SM1.5 Field-sweep data for $BaFe_2Se_2O$ at 10 K

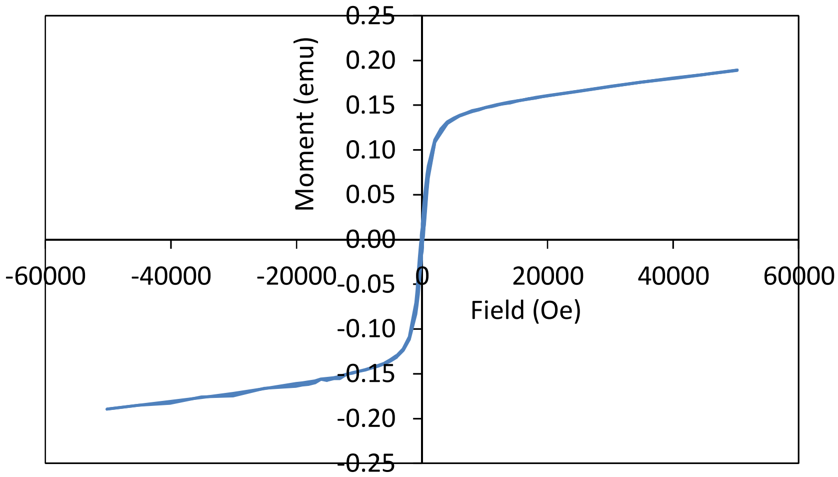


Figure SM1.5 Field-sweep data for $BaFe_2Se_2O$ at 10 K

SM1.6 FC and ZFC data for $BaFe_2Se_2O$ in 45000 Oe applied field

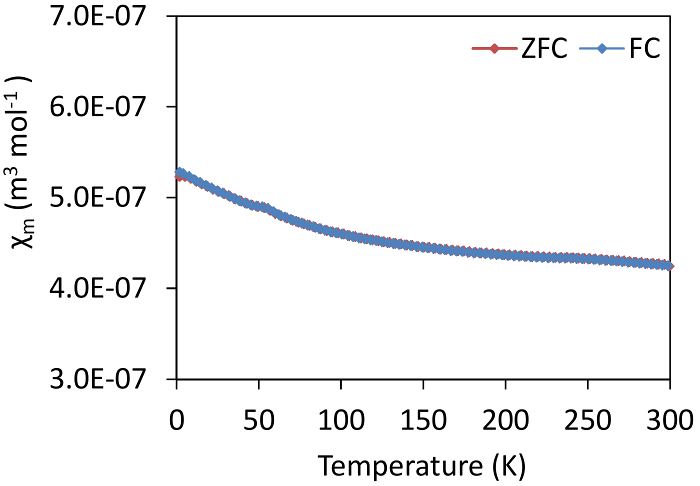


Figure SM1.6 Field-cooled and zero-field-cooled magnetisation data for collected for $BaFe_2Se_2O$ in 45000 Oe applied field.

SM1.7 FC and ZFC data for $BaFe_2Se_2O$ in 37500 Oe applied field

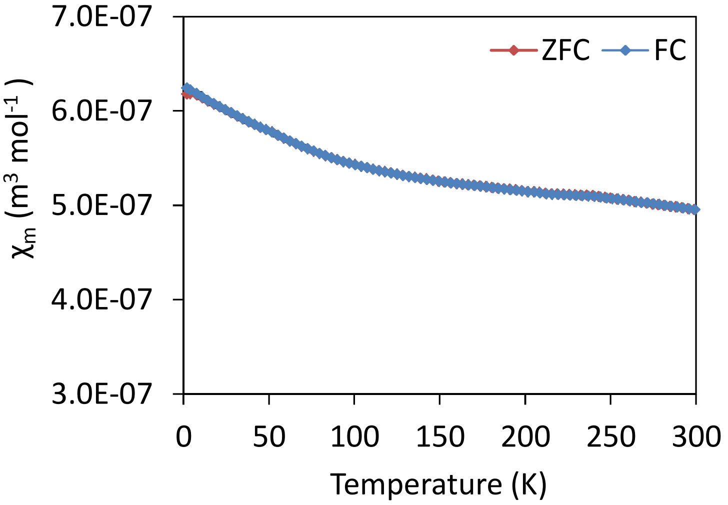


Figure SM1.7 Field-cooled and zero-field-cooled magnetisation data for collected for $BaFe_2Se_2O$ in 37500 Oe applied field.

SM1.8 FC and ZFC data for $BaFe_2Se_2O$ in effective applied field of 7500 Oe

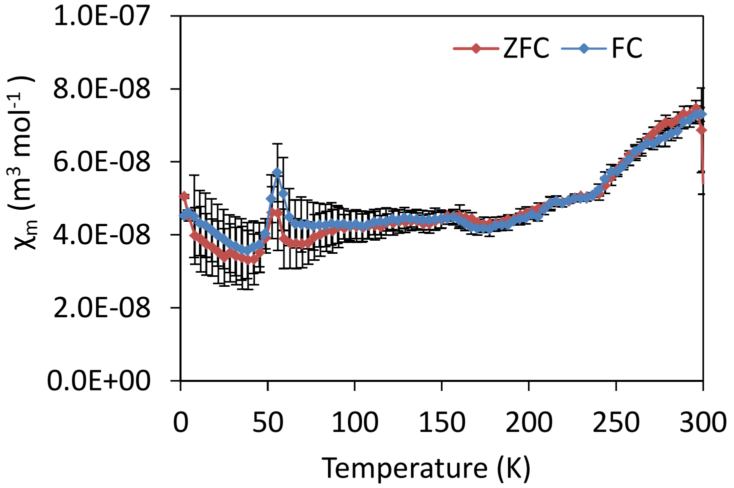


Figure SM1.8 Field-cooled and zero-field-cooled magnetisation data for collected for $BaFe_2Se_2O$ in effective applied field of 7500 Oe.

**SM2 Rietveld refinement data:**

SM2.1 Refinement profiles for $BaFe_2Se_2O$ using 275 K NPD data

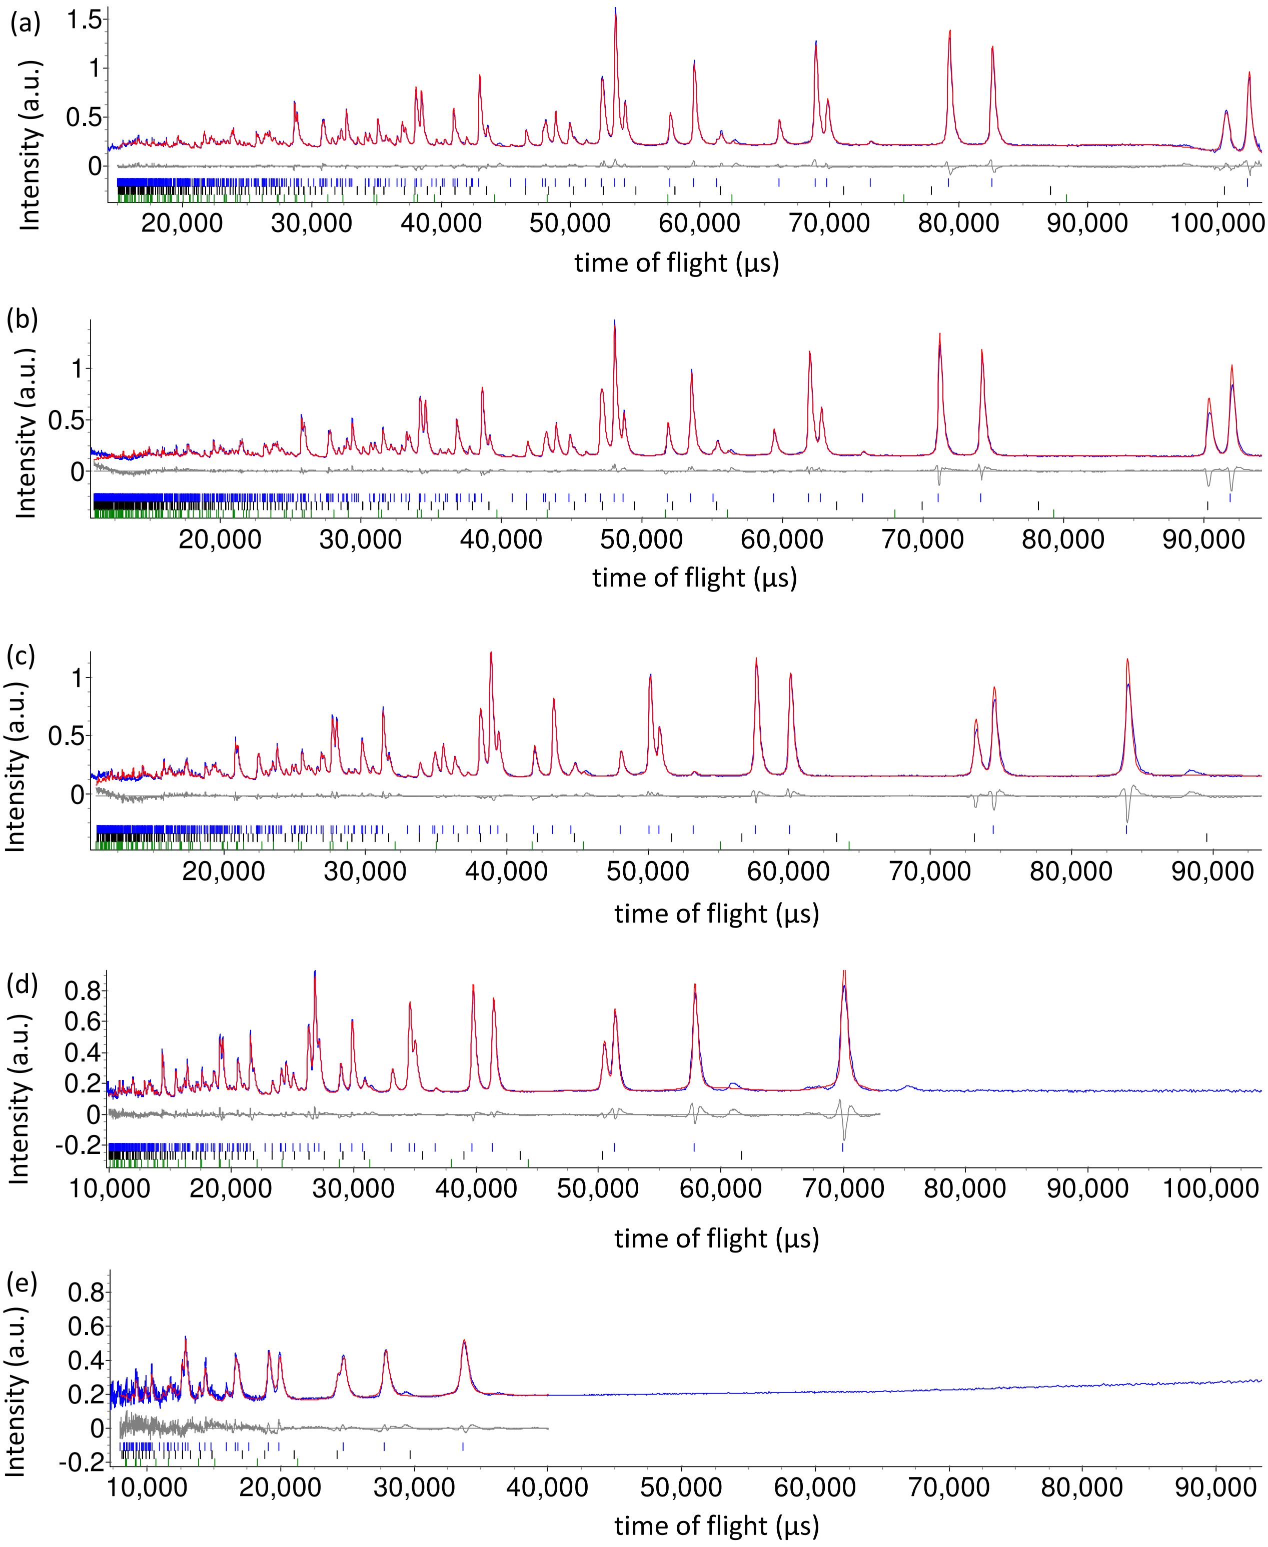


Figure SM2.1 Refinement profiles for $BaFe_2Se_2O$ using 275 K NPD data showing (a) higher resolution (153° bank) data, (b) 122° bank data, (c) 90° bank data, (d) 58° bank data and (e) 27° bank data, with data from lower angle (longer d-spacing banks) in particular showing no evidence for diffuse magnetic scattering at 275 K. Observed, calculated and difference profiles are shown in blue, red and grey, respectively; upper blue ticks, middle black tick and lower green ticks show reflection positions for the $BaFe_2Se_2O$ (94.77(4)% by mass), $Fe_3O_4$ (3.36(2)% by mass), and FeSe (1.86(1)% by mass), respectively.

## SM2.2 Refinement profiles for $BaFe_2Q_2O$ (Q = S, Se) using low temperature NPD data

| | | | ***Q* = S, 1.8 K** | ***Q* = Se, 2 K** |
|---|---|---|---|---|
| | | *a* (Å) | 3.9975(1) | 4.12633(6) |
| | | *b* (Å) | 9.5459(5) | 9.8378(1) |
| | | *c* (Å) | 6.4528(2) | 6.7006(1) |
| | | volume (Å$^3$) | 246.24(2) | 272.005(8) |
| Ba | 2*a* | z | 0.5310(7) | 0.5115(2) |
| | | $U_{iso}$ ×100 (Å$^2$) | 1.3(2) | 0.30(5) |
| Fe | 4*e* | y | 0.6658(3) | 0.66373(5) |
| | | z | 0.8820(3) | 0.88166(8) |
| | | $U_{iso}$ ×100 (Å$^2$) | 1.3(2) | 0.82(3) |
| | | Fe moment ($\mu_B$) | 3.15(3) | 3.31(1) |
| Se | 4*e* | y | 0.7823(9) | 0.79222(6) |
| | | z | 0.757(1) | 0.75777(9) |
| | | $U_{iso}$ ×100 (Å$^2$) | 1.3(2) | 0.63(4) |
| O | 2*b* | z | 0.7311(8) | 0.7385(1) |
| | | $U_{iso}$ ×100 (Å$^2$) | 1.3(2) | 0.59(5) |
| | | Fe – Fe [010] (Å) | 3.166(6) | 3.222(1) |
| | | Fe – Fe [111] (Å) | 2.983(4) | 3.1069(7) |
| | | Fe – O (Å) | 1.858(4) | 1.8749(7) |
| | | Fe – *Q* [001] (Å) | 2.382(8) | 2.4546(8) |
| | | Fe – *Q* [110] (Å) | 2.426(5) | 2.5581(4) |
| | | Fe – O – Fe (°) | 116.8(3) | 118.43(7) |
| | | Fe – *Q* – Fe [100] (°) | 111.0(3) | 107.52(2) |
| | | Fe – *Q* – Fe [111] (°) | 76.7(2) | 76.57(2) |
| | | $R_{wp}$ (%) | 3.80 | 3.39 |
| | | $R_p$ (%) | 2.86 | 3.99 |
| | | $\chi^2$ | 13.25 | 12.24 |

Table SM2.2 Refinement details and selected distances, bond lengths and angles from Rietveld refinements using 1.8 K NPD data for $BaFe_2S_2O$ and 2 K NPD data for $BaFe_2Se_2O$ using *Pmmn* nuclear model and Γ1-magnetic model with no canting (moments along [010]) for both.

## SM2.3 Refinement profiles for $BaFe_2S_2O$ using 2 K NPD data

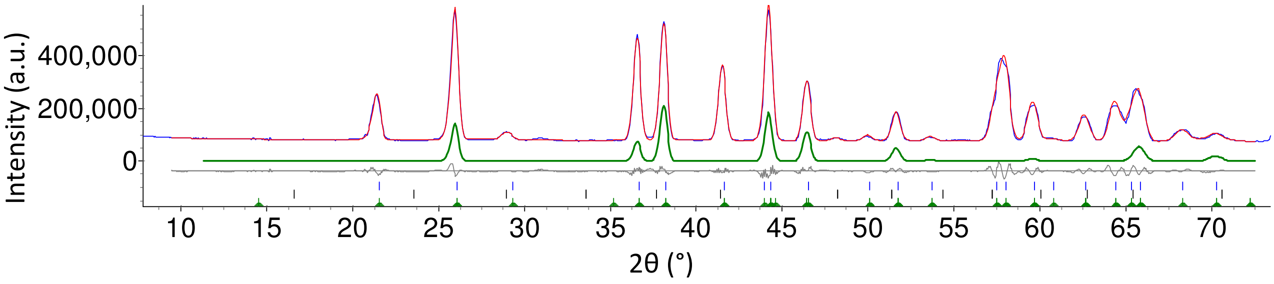


Figure SM2.3 Refinement profiles for $BaFe_2S_2O$ using 2 K NPD data. Observed, calculated and difference profiles are shown in blue, red and grey, respectively; upper blue ticks, middle black ticks and lower green ticks show reflection positions for $BaFe_2S_2O$, $Fe_3O_4$ and the Γ1- magnetic phase with no canting (moments along [010]), respectively, and scattering from the magnetic phase is highlighted in green.

SM2.4 Refinement profiles for $BaFe_2Se_2O$ using 2 K NPD data

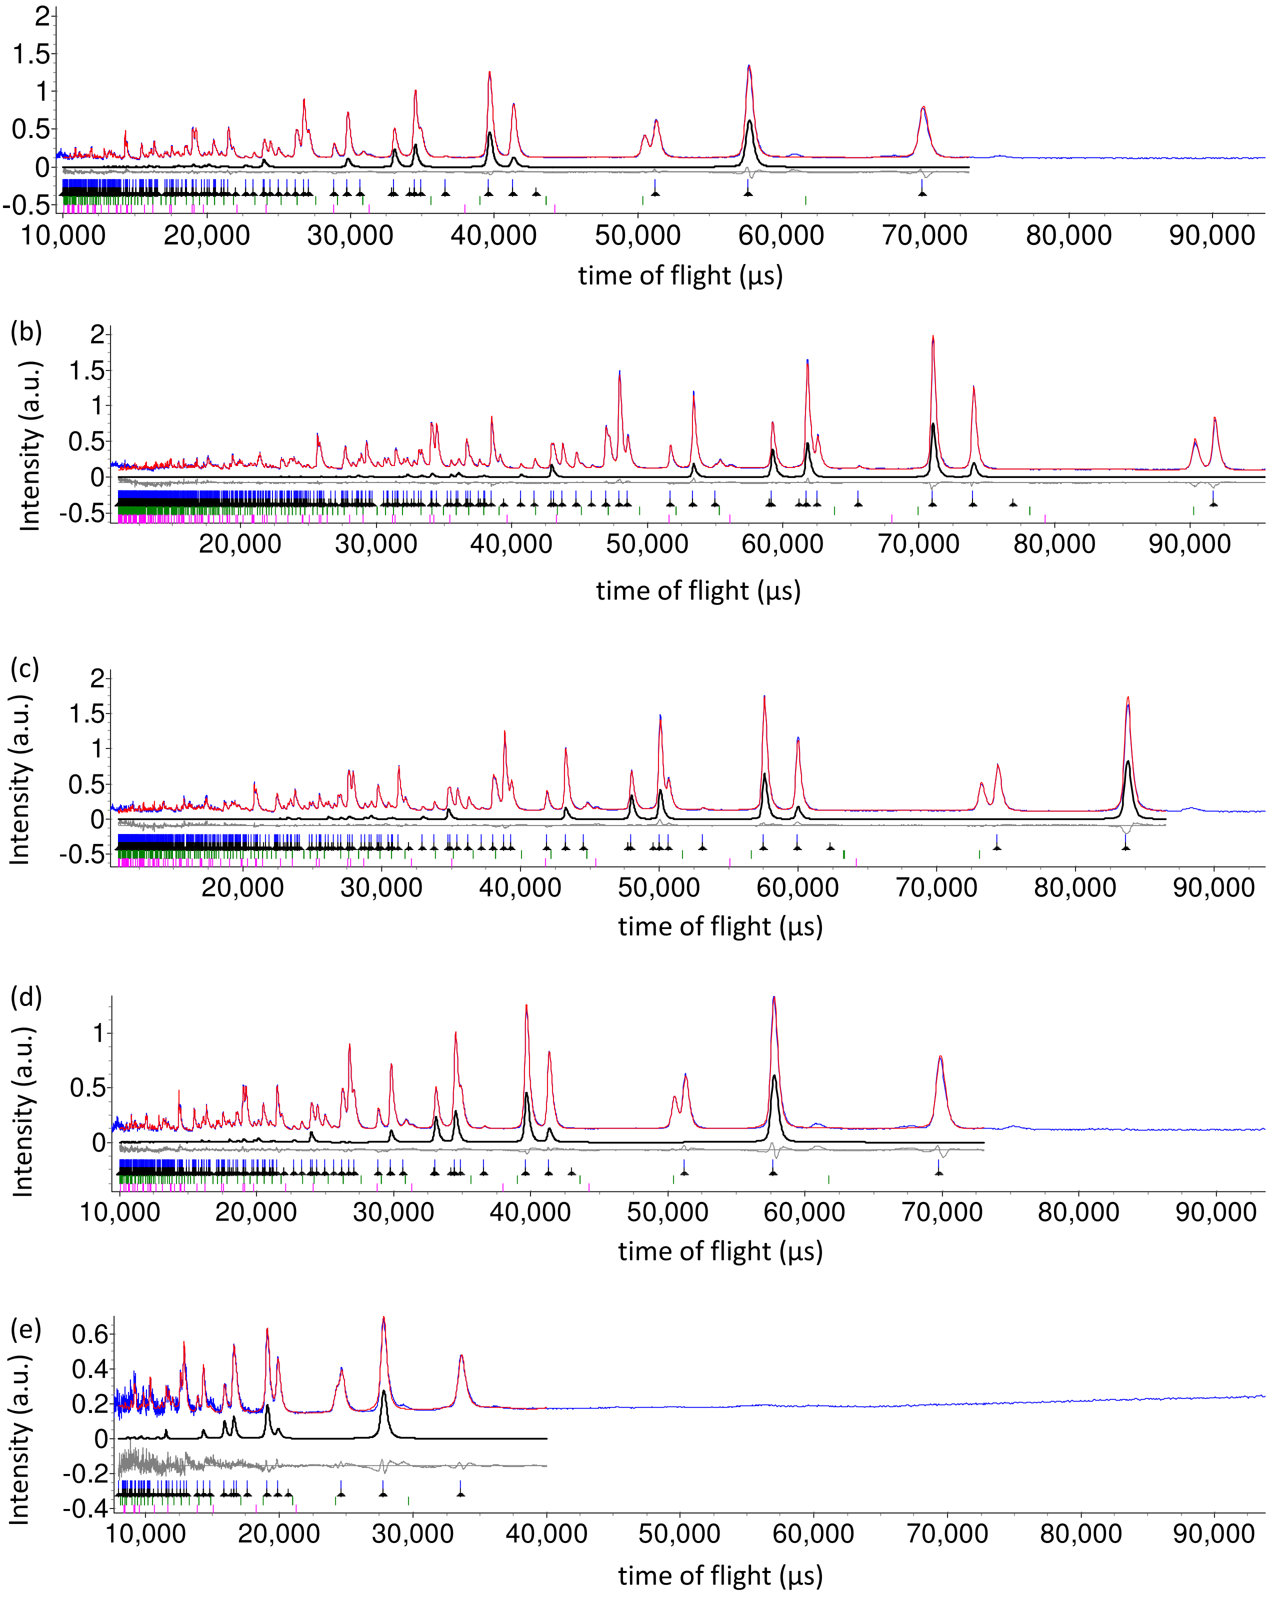


Figure SM2.4 Refinement profiles for $BaFe_2Se_2O$ using 2 K NPD data showing (a) higher resolution (153° bank) data, (b) 122° bank data, (c) 90° bank data, (d) 58° bank data and (e) 27° bank data, with data from lower angle (longer d-spacing banks). Observed, calculated and difference profiles are shown in blue, red and grey, respectively; upper blue ticks, middle black ticks, middle green ticks and bottom pink ticks show reflection positions for $BaFe_2Se_2O$, the Γ1- magnetic phase with no canting (moments along [010]), $Fe_3O_4$ and FeSe, respectively.

SM2.5 Results from analysis NPD data collected on warming for $BaFe_2S_2O$ showing unit cell parameters and intensities of magnetic Bragg reflections with temperature.

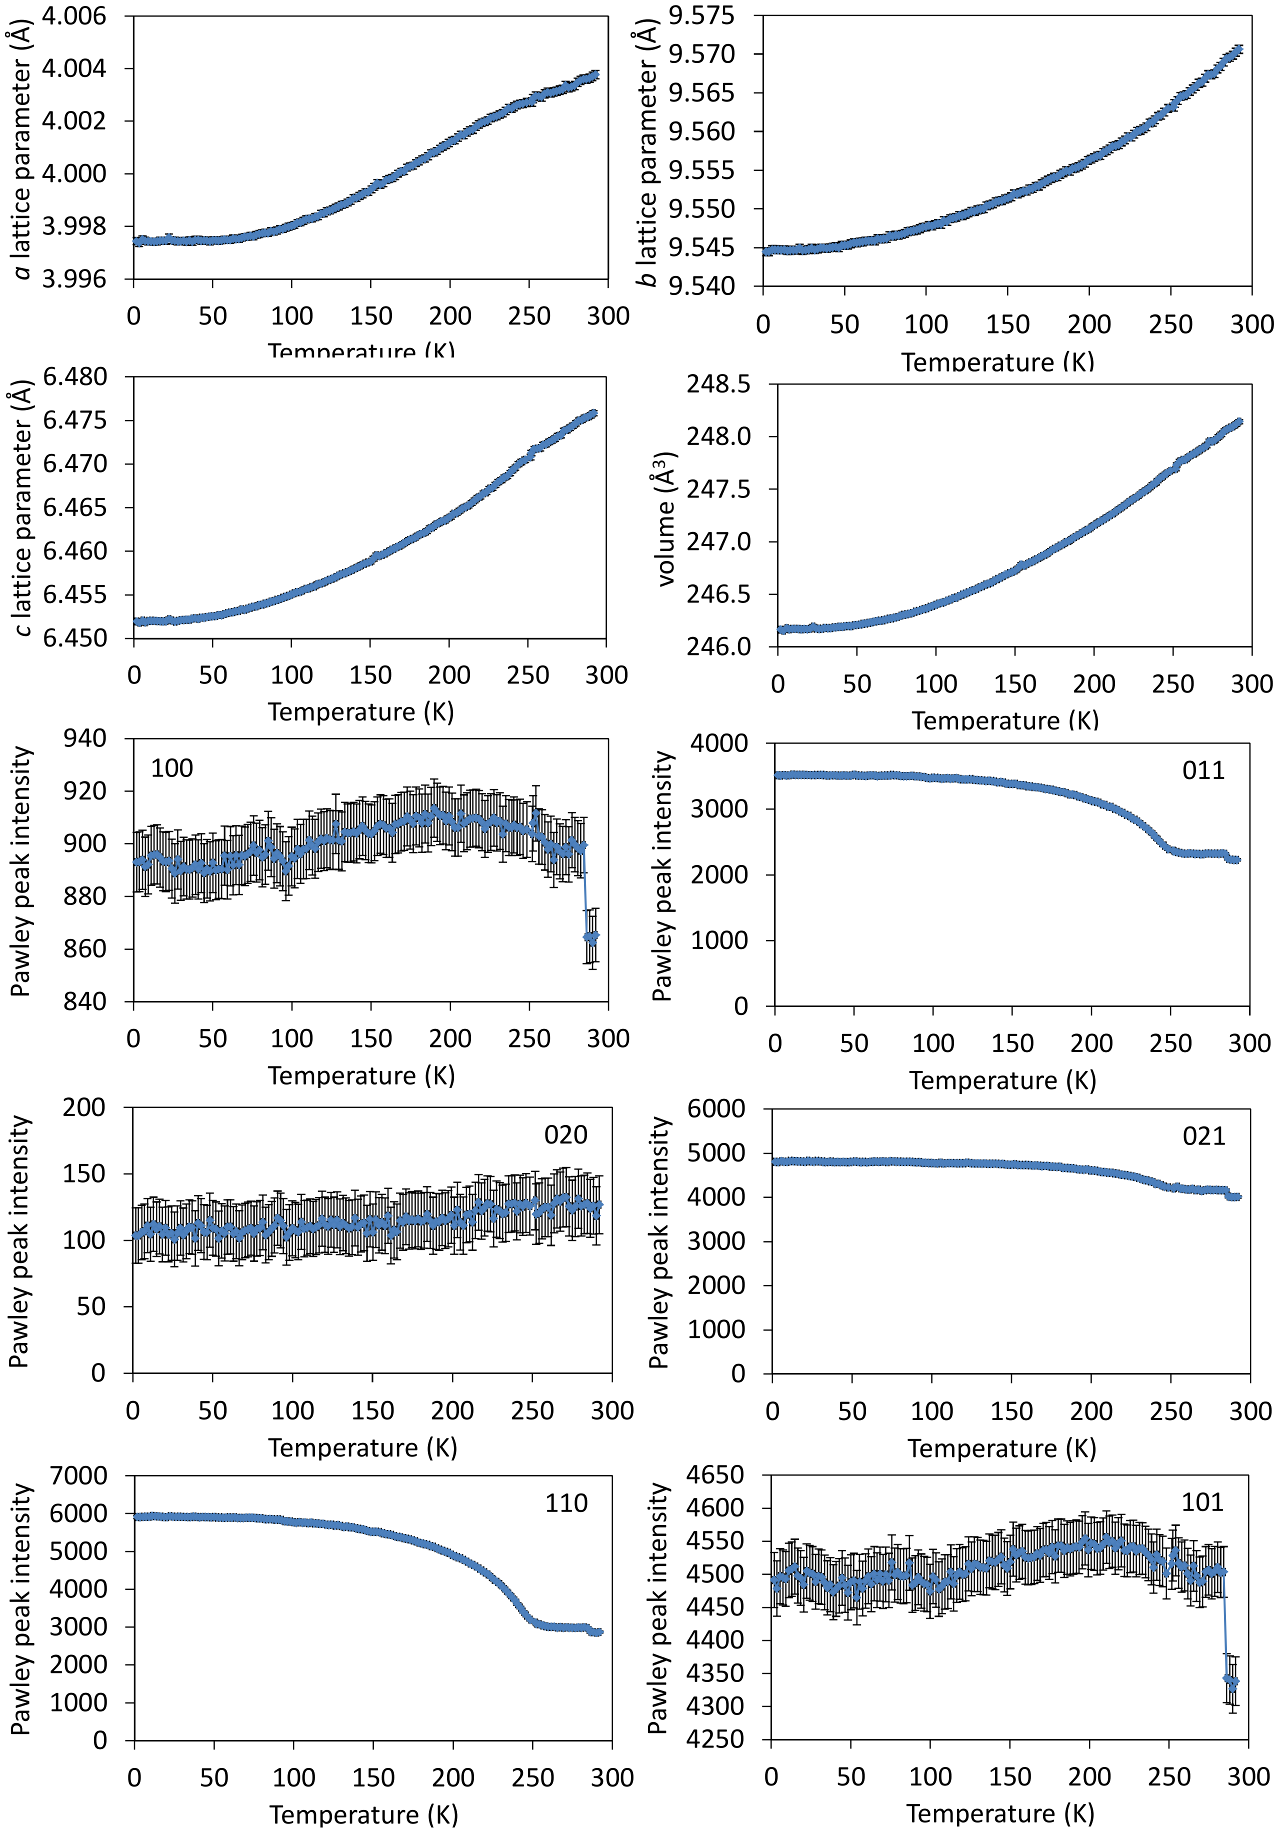

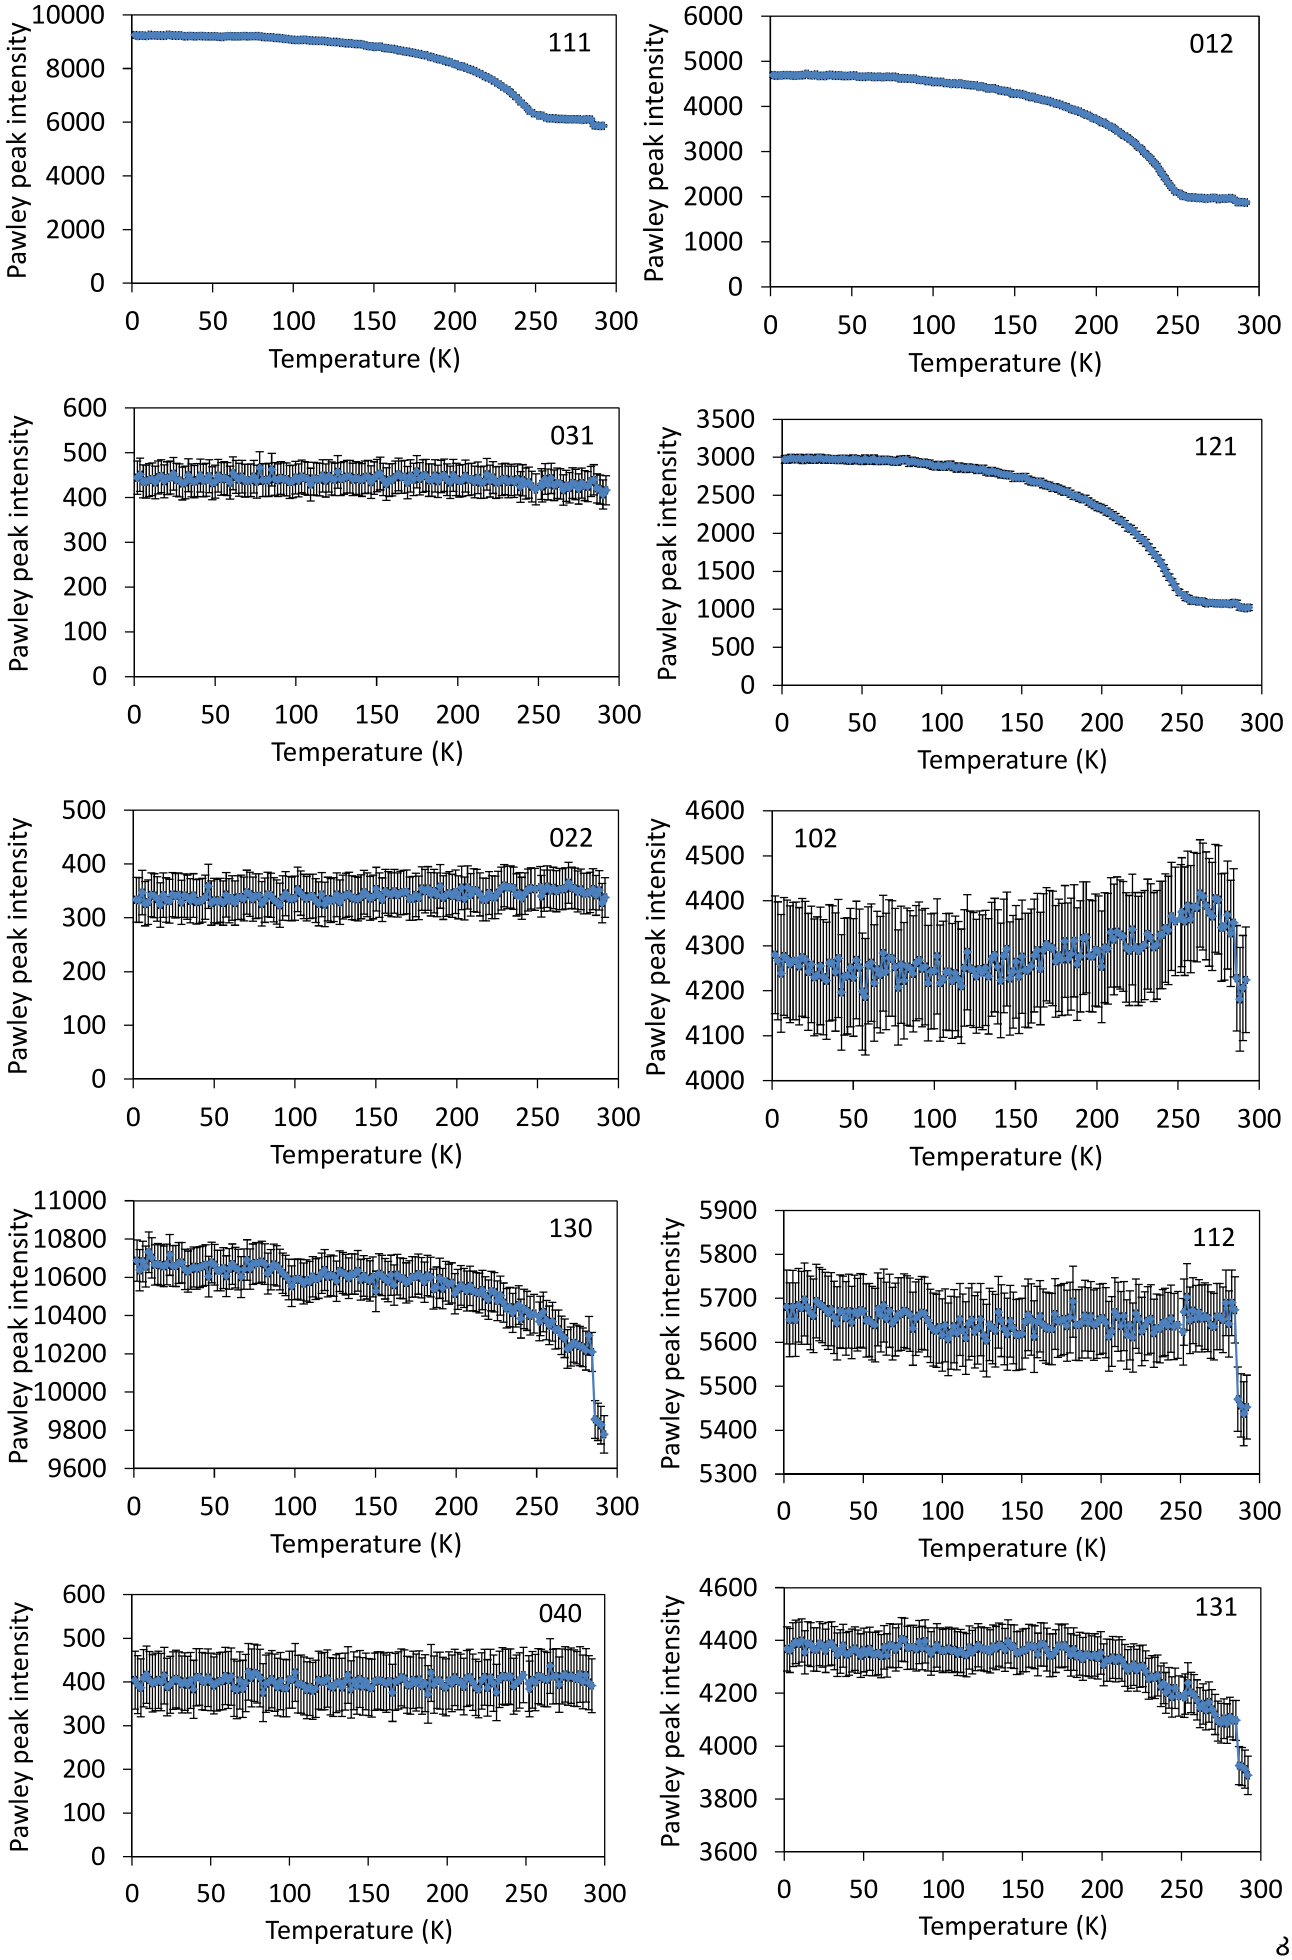
111
012
031
121
022
102
130
112
040
131
Pawley peak intensity
Temperature (K)

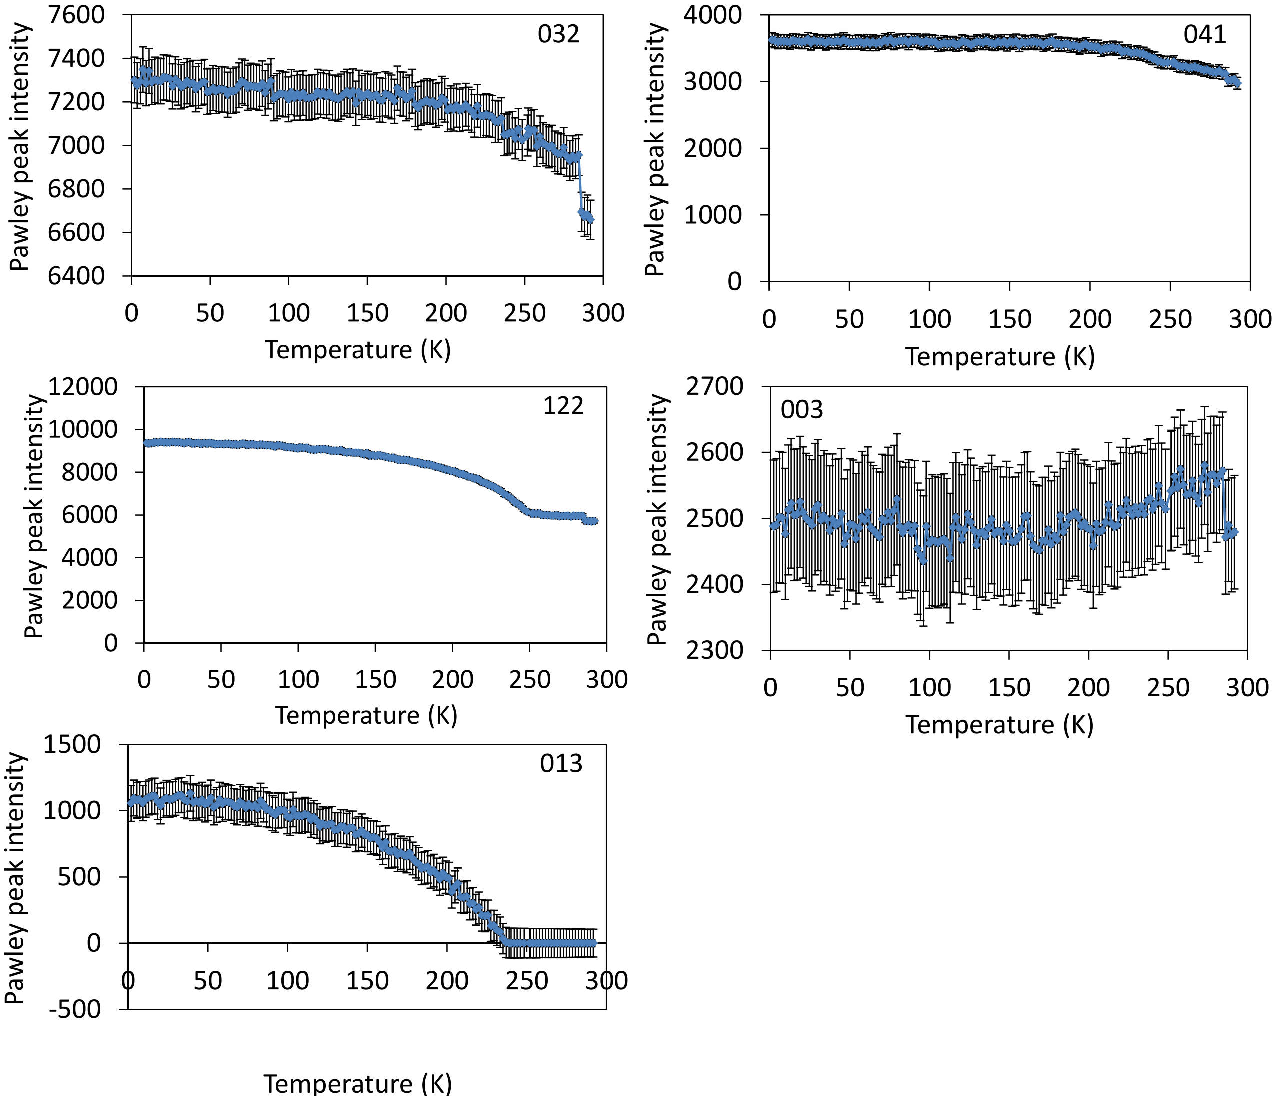


Figure SM2.5 Unit cell parameters and magnetic peak intensities for $BaFe_2S_2O$ from sequential refinements using variable temperature NPD data.

SM2.6 Results from analysis NPD data collected on warming for $BaFe_2Se_2O$ showing unit cell parameters and selected bond lengths and angles with temperature.

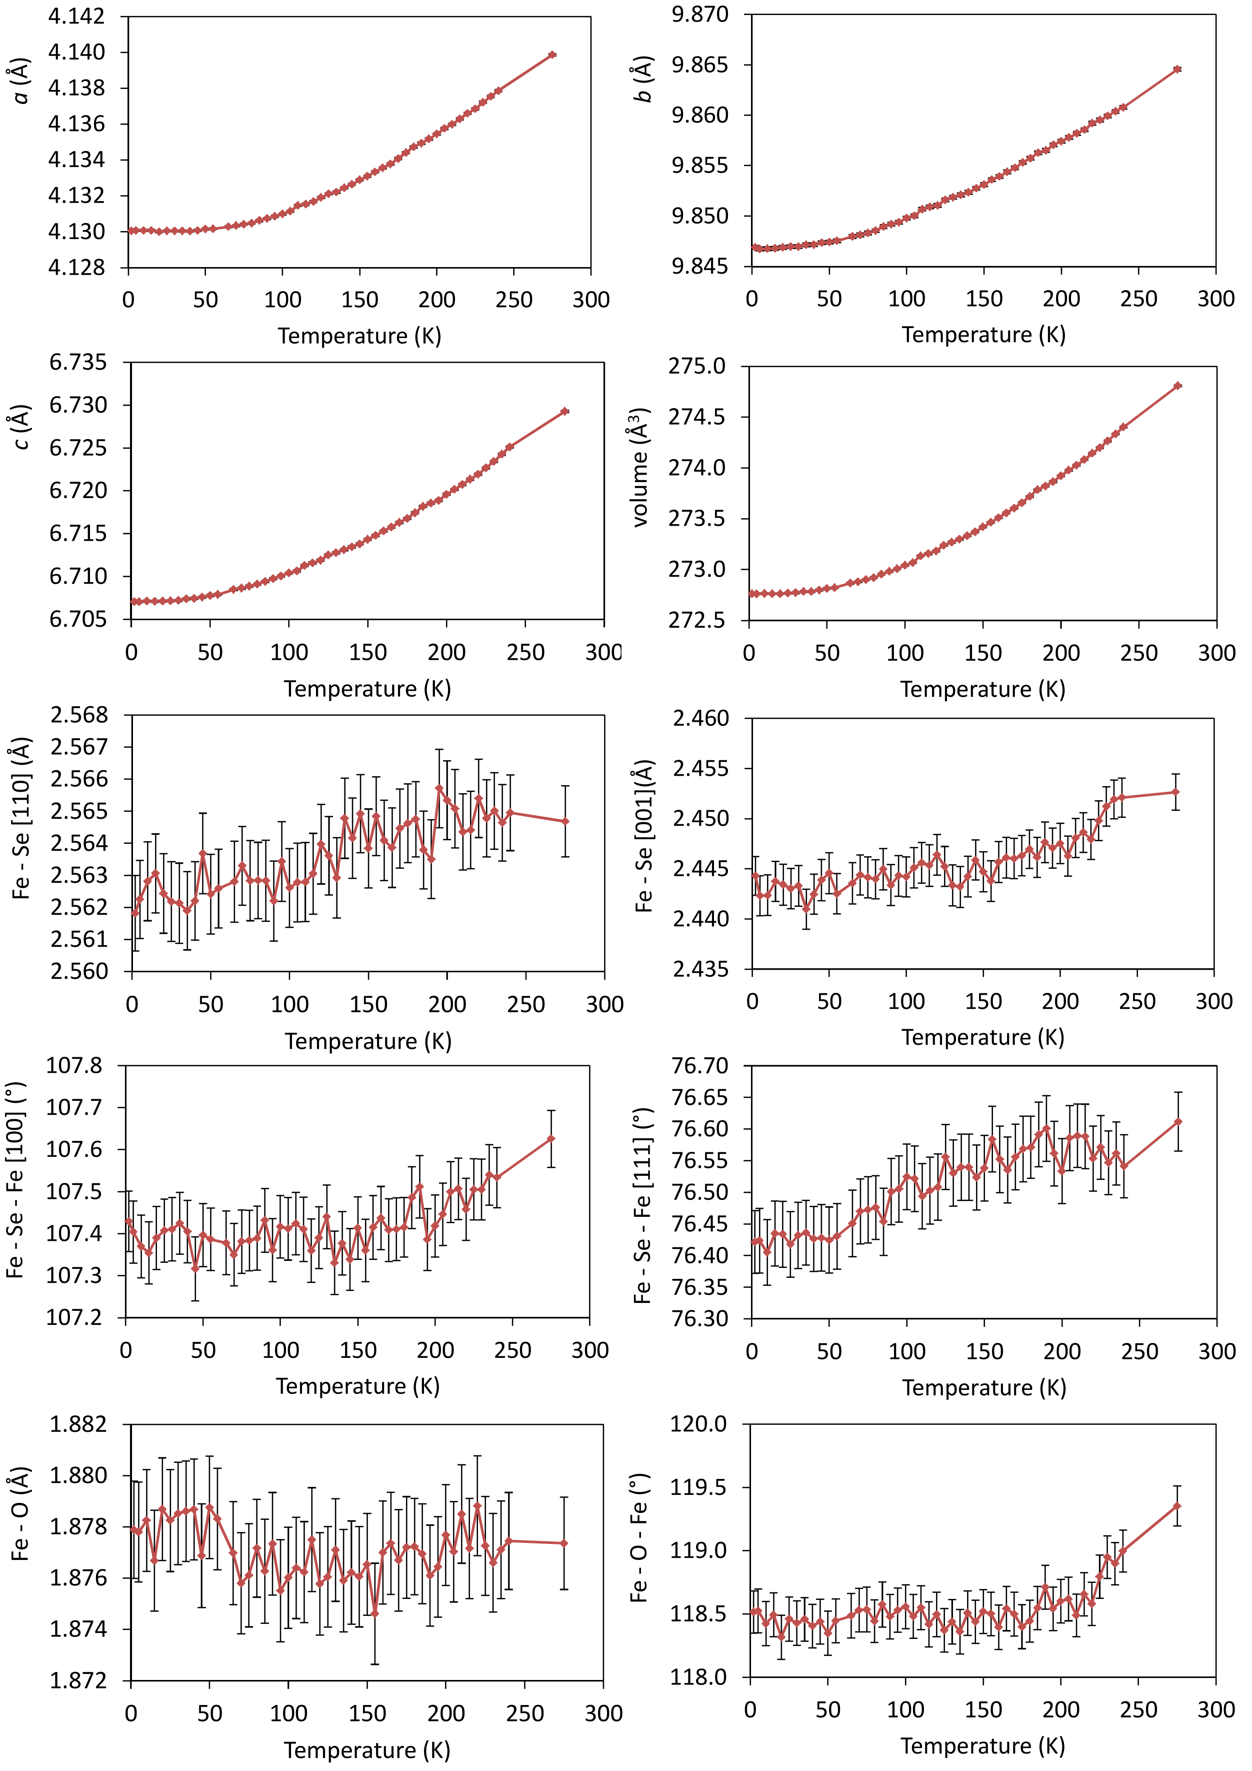

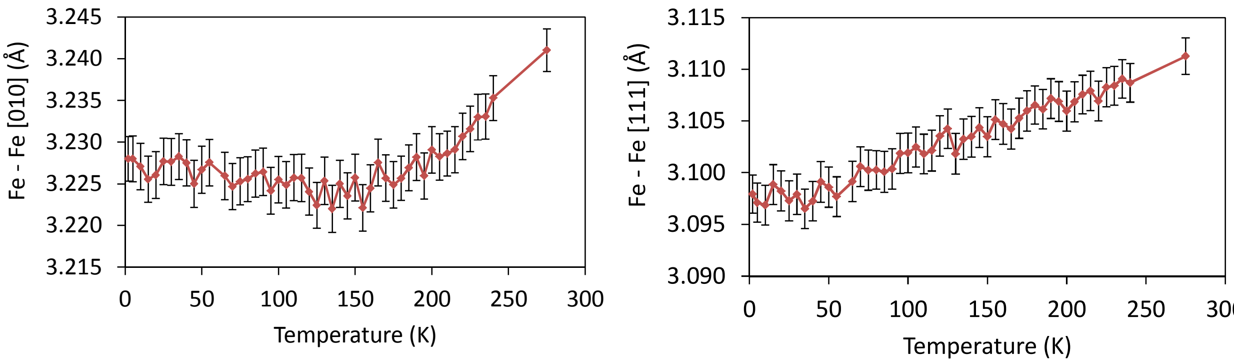


Figure SM2.6 Unit cell parameters and selected distances, bond angles and lengths for $BaFe_2Se_2O$ from sequential refinements using variable temperature NPD data.

SM2.7 Evolution of magnetic ordering for $BaFe_2Se_2O$ and $BaFe_2S_2O$ from analysis NPD data collected on warming.

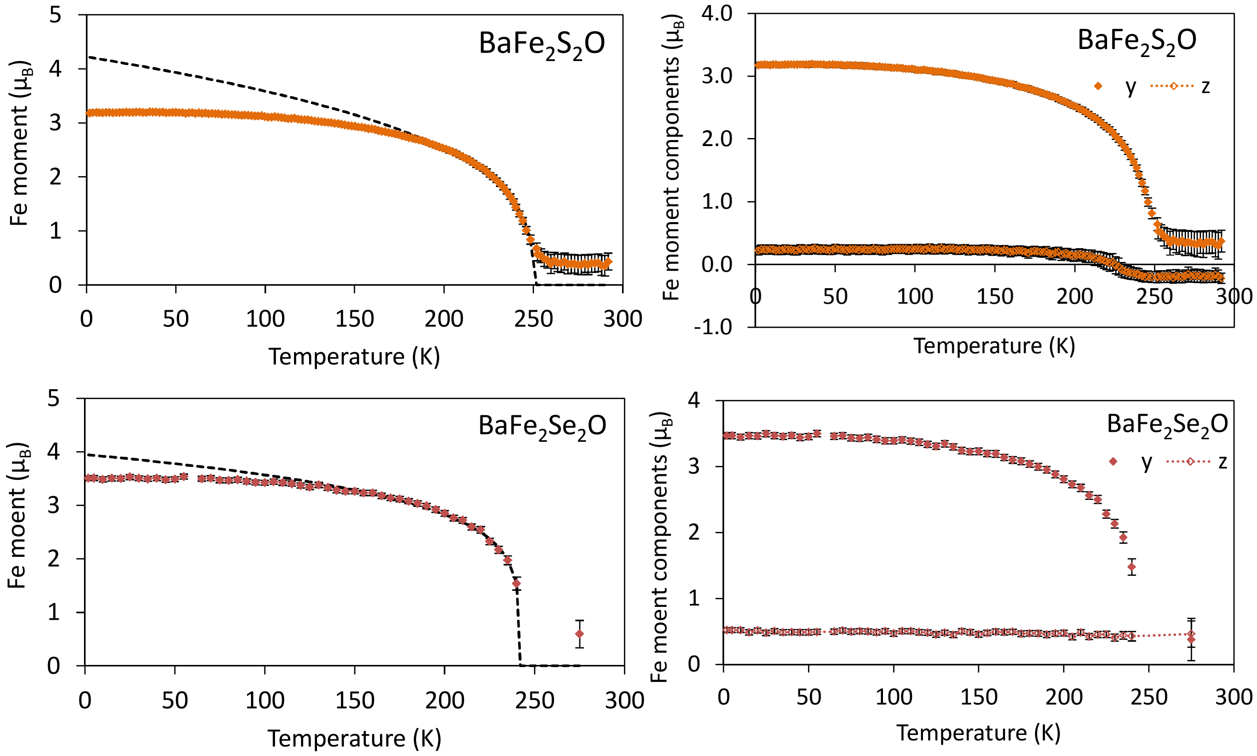


Figure SM2.7 Evolution of magnetic moments for $BaFe_2S_2O$ (above) and $BaFe_2Se_2O$ (below) from sequential refinements using variable temperature NPD data.

SM2.8 Refinement profiles for $BaFe_2Se_2O$ using 2 K NPD data.

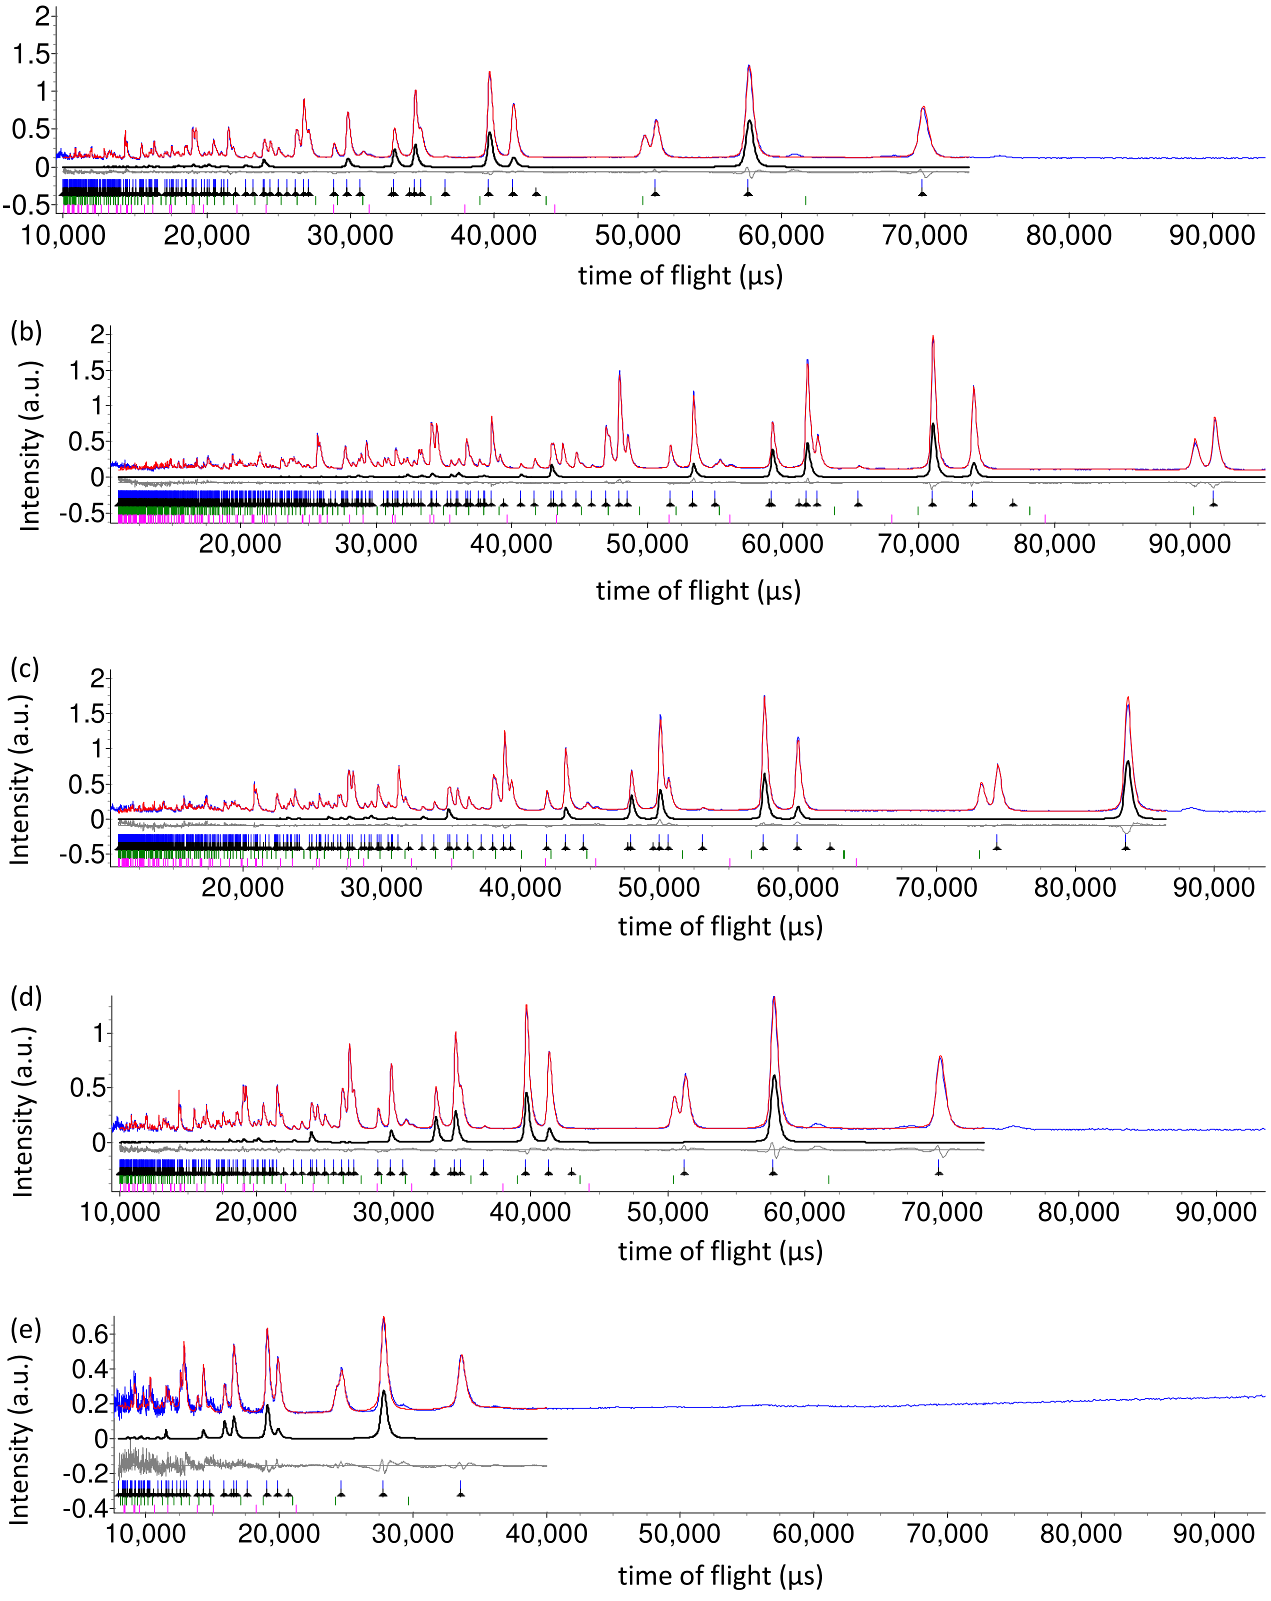


Figure SM2.8 Refinement profiles for $BaFe_2Se_2O$ using 2 K NPD data showing (a) higher resolution (153° bank) data, (b) 122° bank data, (c) 90° bank data, (d) 58° bank data and (e) 27° bank data, with data from lower angle (longer d-spacing banks). Observed, calculated and difference profiles are shown in blue, red and grey, respectively; upper blue ticks, middle black ticks, middle green ticks and bottom pink ticks show reflection positions for $BaFe_2Se_2O$, the magnetic-only phase (allowing canting of the moments), $Fe_3O_4$ and FeSe, respectively.

## SM3 Density functional theory calculations:

### SM3.1 Magnetic models (shown in Figure 5) and their relative energies

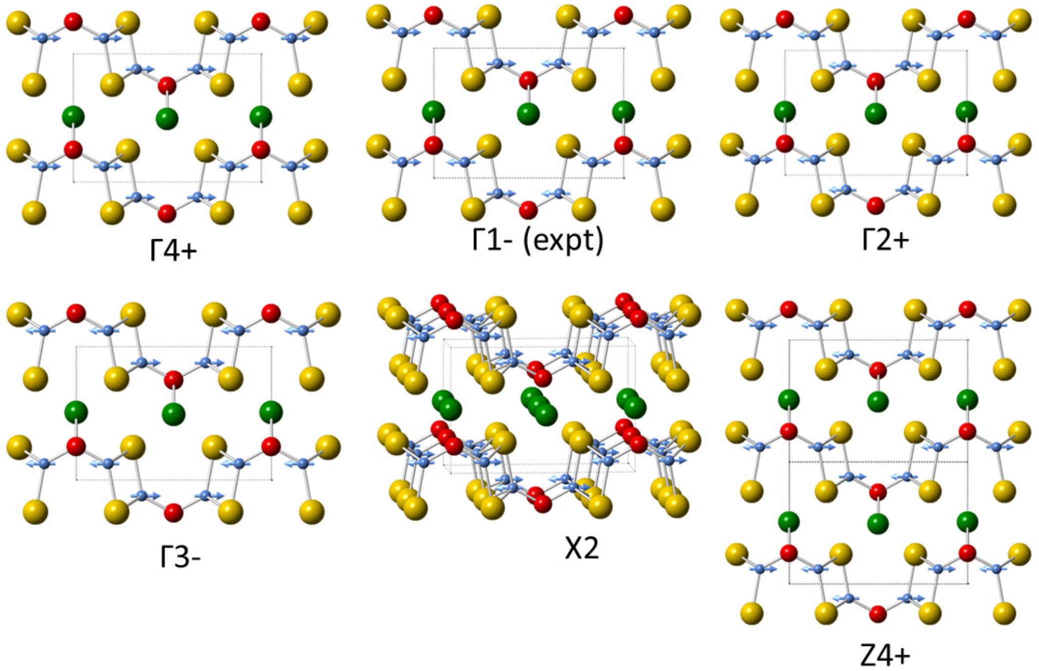


Figure SM3.1 Magnetic models used in DFT calculations

| Magnetic model | Ground state energy |
|---|---|
| FM (Γ4+) | $E_{FM} = 4(-2J_1 - 4J_2 - 4J_3 - 4J_4)$ |
| Γ1- (expt) | $E_{\Gamma1-} = 4(2J_1 - 4J_2 + 4J_3 - 4J_4)$ |
| Γ2+ | $E_{\Gamma2+} = 4(2J_1 - 4J_2 - 4J_3 - 4J_4)$ |
| Γ3- | $E_{\Gamma3-} = 4(-2J_1 - 4J_2 + 4J_3 - 4J_4)$ |
| X2 | $E_{X2} = 4(2J_1 + 4J_2 - 4J_4)$ |
| Z4+ | $E_{Z4+} = 4(2J_1 - 4J_2 - 4J_3 + 4J_4)$ |

Table SM3.1 Ground state energies (in terms of exchange interaction $J_n$) for magnetic models used in DFT calculations.

| U (eV) | $BaFe_2S_2O$ | | | $BaFe_2Se_2O$ | | |
|---|---|---|---|---|---|---|
| | Maximum force (eV/Å) | Pressure (kbar) | Magnetic moment (μB) | Maximum force (eV/Å) | Pressure (kbar) | Magnetic moment (μB) |
| 2.0 | 0.6 | -16.6 | 3.3 | 0.2 | -14.6 | 3.3 |
| 3.5 | 0.4 | 3.3 | 3.4 | 0.1 | 2.0 | 3.4 |
| 5.0 | 0.4 | 19.6 | 3.5 | 0.3 | 15.5 | 3.6 |
| 6.5 | 0.6 | 33.1 | 3.6 | 0.5 | 26.7 | 3.6 |

Table SM3.2 Maximum force on any ion, total external pressure on unit cell and magnetic moments for the Γ1- magnetic model from DFT calculations using the experimental crystal structure.

1. Lei, H.; Ryu, H.; Ivanovski, V.; Warren, J. B.; Frenkel, A. I.; Cekic, B.; Yin, W.-G.; Petrovic, C., Structure and physical properties of the layered iron oxychalcogenide BaFe2Se2O. *Phys. Rev. B* **2012,** *86*, 195133.
